# Supplementary material for: Giant Phonon Anomaly associated with Superconducting Fluctuations in the Pseudogap Phase of Cuprates
Source: arXiv:1506.01258 source file (2015-06-03)
Supplement: Supplementary file 1 [file SI.pdf]

# Giant Phonon Anomaly associated with Superconducting Fluctuations in the Pseudogap Phase of Cuprates

**Contents**


**I. Derivation of the Leggett mode** 2
A. Fluctuation region 2
B. Ordered region $T = 0$ 4

**II. Calculation of the phonon self energy** 5
A. Summation of subband indices 5
B. Intermediate state in fluctuation region 5
C. Intermediate state in ordered region $T = 0$ 7
D. Numerical calculation for $B$ in the fluctuation region 8

**References** 8

## I. DERIVATION OF THE LEGGETT MODE

### A. Fluctuation region

As in the main text, the propagator for superconducting fluctuations is derived by the following Bethe-Salpeter equation (see Fig. 1)

$$\begin{aligned} L_{pp'q} &= \gamma_{\mathbf{p}} L_q \gamma_{\mathbf{p}'} = \gamma_{\mathbf{p}} \begin{pmatrix} U & J \\ J & U \end{pmatrix} \gamma_{\mathbf{p}'} - \gamma_{\mathbf{p}} \begin{pmatrix} U & J \\ J & U \end{pmatrix} \begin{pmatrix} \pi_a(q) & 0 \\ 0 & \pi_b(q) \end{pmatrix} L_q \gamma_{\mathbf{p}'}, \\ \pi_i(q) &= \frac{1}{\beta V} \sum_{\mathbf{p}\in S_i} \sum_{i\omega} \gamma_{\mathbf{p}}^2 G\left(\frac{\mathbf{q}}{2} + \mathbf{p}, iq_0 + i\omega\right) G\left(\frac{\mathbf{q}}{2} - \mathbf{p}, -i\omega\right), \end{aligned} \tag{1}$$

where $q = (\mathbf{q}, iq_0)$, and similarly for $p$ and $p'$. Note that $U < 0$ and $J < 0$ are both attractive in our notation. $\mathbf{p} \in S_i$ means the summation over momentum is restricted to the $i$th subband. Taking into account the strong damping of the quasiparticles in the underdoped regime, we assume a phenomenological form of the electron Green's function

$$\begin{aligned} G(\mathbf{p}, i\omega) &= \frac{1}{i\omega - \epsilon_{\mathbf{p}} + i\Gamma^{(e)}\mathrm{sgn}\omega}, \\ \Gamma^{(e)} &= aT + bT^2, \end{aligned} \tag{2}$$

where a quadratic temperature dependence of the quasiparticle damping rate is used according to transport studies [1]. To calculate $\pi$, we follow the general procedure of superconducting fluctuation theory [2, 3]. For any bosonic frequency $\omega_k > 0$, we have

$$\pi_i(\mathbf{q}, i\omega_k) \approx N_0 \sum_{n\geq 0} \left\langle \gamma_{\mathbf{p}}^2 \left[ \frac{1}{n + \frac{1}{2} + \frac{\omega_k}{4\pi T} + \frac{\Gamma^{(e)}}{2\pi T}} - \frac{1}{(4\pi T)^2} \frac{\left(v_{\mathbf{p}}^F \cdot \mathbf{q}\right)^2}{\left(n + \frac{1}{2} + \frac{\omega_k}{4\pi T} + \frac{\Gamma^{(e)}}{2\pi T}\right)^3} \right] \right\rangle_i . \tag{3}$$

Here $N_0$ is the density of states per spin at the Fermi level in one subband, $\mathbf{v}_{\mathbf{p}}^F$ is the Fermi velocity at $\mathbf{p}$ in subband $i$. We use $\langle \ldots \rangle_i$ to denote the average over the Fermi surface of subband $i$. A normalized $d$-wave symmetry factor $\gamma_{\mathbf{p}} = \sqrt{2} \cos 2\theta_{\mathbf{p}}$ is chosen, where $\theta_{\mathbf{p}}$ is the angle measured from the center of the arc and $\left\langle \gamma_{\mathbf{p}}^2 \right\rangle_i = 1$. Introducing a large bosonic frequency $\omega_c = 2n_{\max}\pi T$ to cut off the summation of the first term (which is logarithmic divergent), it follows

$$\begin{aligned} \sum_{n\geq 0}^{n_{\max}} \frac{1}{n + \frac{1}{2} + \frac{\omega_k}{4\pi T} + \frac{\Gamma^{(e)}}{2\pi T}} &= \psi\left(\frac{1}{2} + \frac{\omega_k}{4\pi T} + \frac{\Gamma^{(e)}}{2\pi T} + \frac{\omega_c}{2\pi T}\right) - \psi\left(\frac{1}{2} + \frac{\omega_k}{4\pi T} + \frac{\Gamma^{(e)}}{2\pi T}\right), \\ \sum_{n\geq 0} \frac{1}{\left(n + \frac{1}{2} + \frac{\omega_k}{4\pi T} + \frac{\Gamma^{(e)}}{2\pi T}\right)^3} &= -\frac{1}{2}\psi''\left(\frac{1}{2} + \frac{\omega_k}{4\pi T} + \frac{\Gamma^{(e)}}{2\pi T}\right), \end{aligned} \tag{4}$$

where the special function $\psi(x) = d[\log\Gamma(x)]/dx$ is the digamma function. The analytic continuation to real frequency is taken by $\omega_k \to -i\omega$, which leads to

$$\begin{aligned} \frac{1}{N_0}\pi_i^R(\mathbf{q}, \omega) = {} & \psi\left(\frac{1}{2} - \frac{i\omega}{4\pi T} + \frac{a + bT}{2\pi} + \frac{\omega_c}{2\pi T}\right) - \psi\left(\frac{1}{2} - \frac{i\omega}{4\pi T} + \frac{a + bT}{2\pi}\right) \\ & + \frac{1}{2(4\pi T)^2}\psi''\left(\frac{1}{2} - \frac{i\omega}{4\pi T} + \frac{a + bT}{2\pi}\right) \left\langle \gamma_{\mathbf{p}}^2 \left(\mathbf{v}_{\mathbf{p}}^F \cdot \mathbf{q}\right)^2 \right\rangle_i . \end{aligned} \tag{5}$$

The superconducting ordering temperature $T_c$, at which the fluctuation propagator $L^R(\mathbf{q} = 0, \omega = 0)$ diverges, is given by

$$T_c = \frac{\omega_c}{2\pi} \exp\left[-\psi\left(\frac{1}{2} + \frac{a + bT_c}{2\pi}\right)\right] \exp\left(-\frac{1}{N_0|U + J|}\right). \tag{6}$$

Note that finite damping $a, b > 0$ suppresses $T_c$, however in cuprates $U$ is strong enough to still lead to a high $T_c$. When $a = b = 0$, the above equation reduces to the conventional BCS equation $T_c = 1.13\omega_c \exp\left[-1/\left(N_0 |V_{\max}|\right)\right]$,

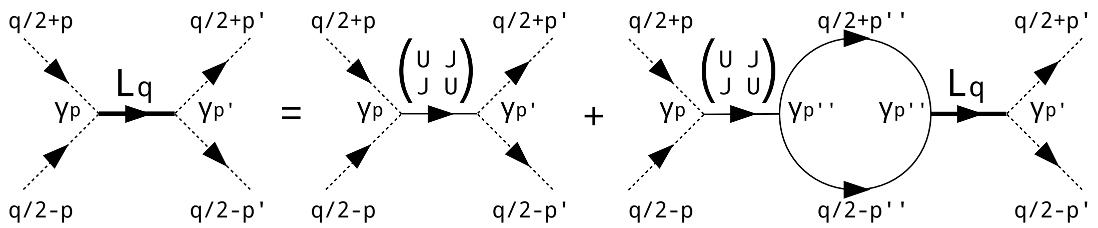


Figure 1: The Bethe-Salpeter equation for the fluctuation propagator. Subband index is implicitly labeled by the matrix subscript.

where $V_{\max}$ is the most attractive interaction, in our two subband case it is the eigenvalue $U+J$ of the bare interaction vertex. In terms of $T_c$, we could rewrite the bubble $\pi$ as

$$\begin{aligned}\frac{1}{N_0}\pi_i^R(\mathbf{q},\omega) &\approx -\frac{1}{N_0(U+J)} - \epsilon + \frac{1}{4\pi T}\psi'\left(\frac{1}{2}+\frac{a+bT_c}{2\pi}\right)[i\omega - 2bT(T-T_c)] \\ &\quad + \frac{1}{2(4\pi T)^2}\psi''\left(\frac{1}{2}+\frac{a+bT}{2\pi}\right)\left\langle \gamma_{\mathbf{p}}^2\left(\mathbf{v}_{\mathbf{p}}^F\cdot\mathbf{q}\right)^2\right\rangle_i, \qquad (7)\end{aligned}$$

where $\epsilon = \log(T/T_c)$ is the reduced temperature.

Solving the Bethe-Salpeter equation (1) for $L^R$, one gets

$$L^R(\mathbf{q},\omega) = \frac{\begin{pmatrix} U + (U^2-J^2)\pi_b^R(\mathbf{q},\omega) & J \\ J & U + (U^2-J^2)\pi_a^R(\mathbf{q},\omega)\end{pmatrix}}{(U^2-J^2)\pi_a^R(\mathbf{q},\omega)\pi_b^R(\mathbf{q},\omega) + U\left[\pi_a^R(\mathbf{q},\omega)+\pi_b^R(\mathbf{q},\omega)\right]+1}. \qquad (8)$$

If we make a further isotropic simplification by averaging over the direction of $\mathbf{q}$ such that $\pi_a^R = \pi_b^R = \pi^R$, then

$$L^R = \frac{\begin{pmatrix} U + (U^2-J^2)\pi^R & J \\ J & U + (U^2-J^2)\pi^R\end{pmatrix}}{[(U+J)\pi^R+1][(U-J)\pi^R+1]} = \left[\frac{P_+}{\pi^R + \frac{1}{U+J}} + \frac{P_-}{\pi^R+\frac{1}{U-J}}\right], \qquad (9)$$

where the two projectors in the nominators are

$$P_\pm = \left(\frac{1}{2} \pm \frac{1}{2}\sigma_x\right). \qquad (10)$$

They satisfy $P_\pm^2 = P_\pm$ and $P_+P_- = 0$. Physically, $P_+$ projects into the subspace of in-phase fluctuations, and $P_-$ into that of out-of-phase fluctuations. The position of the pole in $P_+$ is located at $\mathbf{q}=\omega=0$ when $T=T_c$. Thus it is the fluctuating version of the Anderson-mode pole (with in-phase nature and gapless nature). In the presence of a local superconducting order parameter, the in-phase phase fluctuation is associated with the total charge density modulation, which is prohibited by the long-range Coulomb interaction. As a result we are mainly interested in the out-of-phase fluctuations i.e. the fluctuating version of the Leggett mode with nominator $P_-$

$$L^R(\mathbf{q},\omega) = \frac{T}{cN_0}\frac{P_-}{i\omega - \tau^{-1} - Dq^2}, \qquad (11)$$

where the constant $c = \frac{1}{4\pi}\psi'\left[\frac{1}{2}+\frac{1}{2\pi}(a+bT_c)\right]$. The above propagator has the form of an overdamped bosonic mode. The total relaxation time $\tau$ and diffusion constant $D$ are defined by the following equations

$$\begin{aligned}\tau^{-1} &= \frac{T}{c}\log\frac{T}{T_c} + 2bT(T-T_c) + \frac{T}{cN_0}\frac{2|J|}{U^2-J^2}, \\ Dq^2 &= -\frac{1}{8\pi T}\frac{\psi''\left[\frac{1}{2}+\frac{1}{2\pi}(a+bT)\right]}{\psi'\left[\frac{1}{2}+\frac{1}{2\pi}(a+bT_c)\right]}\left\langle\gamma_{\mathbf{p}}^2\left(\mathbf{v}_{\mathbf{p}}^F\cdot\mathbf{q}\right)^2\right\rangle \\ &= -\frac{v_F^2}{16\pi T}\frac{\psi''\left[\frac{1}{2}+\frac{1}{2\pi}(a+bT)\right]}{\psi'\left[\frac{1}{2}+\frac{1}{2\pi}(a+bT_c)\right]}q^2, \qquad (12)\end{aligned}$$

where in the expression for $D$, the symbol $\langle\ldots\rangle$ means averaging over both the directions of $\mathbf{p}$ and $\mathbf{q}$, and the result is independent on the subband index $i$. From now on we denote the total damping of Leggett mode to be

$$\Gamma_{\mathbf{q}}^{(\mathrm{LM})}=\tau^{-1}+Dq^{2}, \tag{13}$$

which leads to the simple expression used in the main text

$$L^{R}\left(\mathbf{q},\omega\right)=\frac{T}{cN_{0}}\frac{1}{i\omega-\Gamma_{\mathbf{q}}^{(\mathrm{LM})}}\left(\frac{1}{2}-\frac{1}{2}\sigma_{x}\right). \tag{14}$$

### B. Ordered region $T=0$

In this case, the structure of the Bethe-Salpeter equation is unchanged, but the electronic bubble receives another contribution from the anomalous Green's function [4–6]. Also the Green's functions change form in the superconducting phase, $G_{p}=\left(ip_{0}+\epsilon_{\mathbf{p}}\right)/\left[\left(ip_{0}\right)^{2}-E_{\mathbf{p}}^{2}\right]$ and $F_{p}=\Delta_{\mathbf{p}}/\left[\left(ip_{0}\right)^{2}-E_{\mathbf{p}}^{2}\right]$, with $E_{\mathbf{p}}=\sqrt{\epsilon_{\mathbf{p}}^{2}+\Delta_{\mathbf{p}}^{2}}$ the quasiparticle energy. We generalize the derivation by Leggett for $s$-wave superconductors [4] to the $d$-wave case. In the following equations, the $\mathbf{q}$-dependent quantities are $\epsilon_{\mathbf{p}\pm\frac{\mathbf{q}}{2}}$, $E_{\mathbf{p}\pm\frac{\mathbf{q}}{2}}$, and $\Delta_{\mathbf{p}\pm\frac{\mathbf{q}}{2}}$. Because $|\mathbf{q}|\ll2\pi$ is small and $|\partial_{\mathbf{p}}\epsilon_{\mathbf{p}}|\gg|\partial_{\mathbf{p}}\Delta_{\mathbf{p}}|$, we set $\Delta_{\mathbf{p}\pm\frac{\mathbf{q}}{2}}\approx\Delta_{\mathbf{p}}=\gamma_{\mathbf{p}}\Delta$. Then it follows

$$\begin{aligned}\pi_{i}\left(q\right) &= \frac{1}{\beta V}\sum_{\mathbf{p}\in S_{i}}\sum_{ip_{0}}\gamma_{\mathbf{p}}^{2}\left[G\left(\frac{\mathbf{q}}{2}+\mathbf{p},iq_{0}+ip_{0}\right)G\left(\frac{\mathbf{q}}{2}-\mathbf{p},-ip_{0}\right)+F\left(\frac{\mathbf{q}}{2}+\mathbf{p},iq_{0}+ip_{0}\right)F\left(\frac{\mathbf{q}}{2}-\mathbf{p},-ip_{0}\right)\right]\\ &\approx N_{0}\int d\epsilon_{\mathbf{p}}\left\langle\gamma_{\mathbf{p}}^{2}\frac{\tanh\frac{E_{\mathbf{p}}}{2T}}{2E_{\mathbf{p}}}\right\rangle_{i}-N_{0}\left\langle\frac{\left(iq_{0}\right)^{2}-\left(\mathbf{v}_{\mathbf{p}}^{F}\cdot\mathbf{q}\right)^{2}}{2\Delta^{2}}\frac{\Delta_{\mathbf{p}}^{2}}{2E_{\mathbf{p}}}\frac{\partial}{\partial E_{\mathbf{p}}}\left(\int d\epsilon_{\mathbf{p}}\frac{\tanh\frac{E_{\mathbf{p}}}{2T}}{2E_{\mathbf{p}}}\right)\right\rangle_{i}.\end{aligned} \tag{15}$$

Here we have taken the leading order term of $q$ and used the identity

$$\int d\epsilon_{\mathbf{p}}\sum_{ip_{0}}\frac{\frac{1}{2}iq_{0}+ip_{0}+\epsilon_{\mathbf{p}}}{\left[\left(iq_{0}+ip_{0}\right)^{2}-E_{\mathbf{p}+\frac{\mathbf{q}}{2}}^{2}\right]\left[\left(ip_{0}\right)^{2}-E_{\mathbf{p}-\frac{\mathbf{q}}{2}}^{2}\right]}=0, \tag{16}$$

because the integrand is odd under $\epsilon_{\mathbf{p}}\to-\epsilon_{\mathbf{p}}$ and $ip_{0}\to-ip_{0}-iq_{0}$. In zero temperature, the first term in the last line of equation (15) becomes

$$N_{0}\int d\epsilon_{\mathbf{p}}\left\langle\frac{\gamma_{\mathbf{p}}^{2}}{2E_{\mathbf{p}}}\right\rangle_{i}=-\frac{1}{U+J}, \tag{17}$$

which is the gap equation in zero temperature. The energy integral in the second term is

$$\frac{\Delta_{\mathbf{p}}^{2}}{2E_{\mathbf{p}}}\frac{\partial}{\partial E_{\mathbf{p}}}\int d\epsilon_{\mathbf{p}}\frac{1}{2E_{\mathbf{p}}}=-\frac{1}{4}\int d\epsilon_{\mathbf{p}}\frac{\Delta_{\mathbf{p}}^{2}}{E_{\mathbf{p}}^{3}}=-\frac{1}{4}\int d\epsilon_{\mathbf{p}}\frac{\partial}{\partial\epsilon_{\mathbf{p}}}\left(\frac{\epsilon_{\mathbf{p}}}{E_{\mathbf{p}}}\right)=-\frac{1}{2}. \tag{18}$$

After a Wick rotation $iq_{0}\to\omega$ and averaging the direction of $\mathbf{q}$, the zero temperature bubble reads

$$\pi\left(\mathbf{q},\omega\right)=-\frac{1}{U+J}+\frac{N_{0}}{4\Delta^{2}}\left(\omega^{2}-\frac{1}{2}v_{F}^{2}q^{2}\right). \tag{19}$$

Then

$$L\left(\mathbf{q},\omega\right)=\frac{1}{\pi\left(\mathbf{q},\omega\right)+\frac{1}{U-J}}\left(\frac{1}{2}-\frac{1}{2}\sigma_{x}\right)=\frac{4\Delta^{2}}{N_{0}}\frac{1}{\omega^{2}-\omega_{\mathbf{q}}^{2}+i\delta}\left(\frac{1}{2}-\frac{1}{2}\sigma_{x}\right), \tag{20}$$

where the dispersion of Leggett mode is

$$\begin{aligned}\omega_{\mathbf{q}}^{2} &= \omega_{0}^{2}+\frac{1}{2}v_{F}^{2}q^{2},\\ \omega_{0}^{2} &= \frac{4\Delta^{2}}{N_{0}}\frac{2\left|J\right|}{U^{2}-J^{2}}.\end{aligned} \tag{21}$$

## II. CALCULATION OF THE PHONON SELF ENERGY

### A. Summation of subband indices

In the main text, the full expression for the phonon self energy is written as

$$\begin{aligned} \Pi^R(\mathbf{Q},\Omega) &= 4\left[\alpha(\mathbf{Q})\right]^4\left[B^R(\mathbf{Q},\Omega)\right]^2 I^R(\Omega), \\ I^R(\Omega) &= \frac{1}{V^2}\sum_{\mathbf{q},\mathbf{k}} \mathrm{Tr} I^R(\mathbf{q},\mathbf{k},\Omega). \end{aligned} \tag{22}$$

The meaning of the trace Tr in equation (22) is explained as follows. We are interested in the case of $|\mathbf{Q}|$ being large enough to lead to inter-subband transitions. In this case the incoming and outgoing Cooper pairs in the diagram for $B$ are from two subbands, thus $B$ is considered to be off-diagonal in the subband space. The fluctuation propagators, on the other hand, contain intra-subband and inter-subband components. As a result, all possibilities of the arrangements of subband indices sum up to a trace over the product of the two fluctuation propagators

$$\mathrm{Tr}\left[\begin{pmatrix} 0 & B \\ B & 0 \end{pmatrix}\begin{pmatrix} L^{(1)}_{\text{intra}} & L^{(1)}_{\text{inter}} \\ L^{(1)}_{\text{inter}} & L^{(1)}_{\text{intra}} \end{pmatrix}\begin{pmatrix} 0 & B \\ B & 0 \end{pmatrix}\begin{pmatrix} L^{(2)}_{\text{intra}} & L^{(2)}_{\text{inter}} \\ L^{(2)}_{\text{inter}} & L^{(2)}_{\text{intra}} \end{pmatrix}\right] = B^2\mathrm{Tr}\left[\begin{pmatrix} L^{(1)}_{\text{intra}} & L^{(1)}_{\text{inter}} \\ L^{(1)}_{\text{inter}} & L^{(1)}_{\text{intra}} \end{pmatrix}\begin{pmatrix} L^{(2)}_{\text{intra}} & L^{(2)}_{\text{inter}} \\ L^{(2)}_{\text{inter}} & L^{(2)}_{\text{intra}} \end{pmatrix}\right]. \tag{23}$$

### B. Intermediate state in fluctuation region

We use the spectral decomposition for the fluctuation propagator $L$ and the bare phonon Green's function $D$ as follows

$$\begin{aligned} L(\mathbf{q},i\omega) &= \int\frac{dx}{2\pi}\frac{-2\mathrm{Im}L^R(\mathbf{q},x)}{i\omega-x}, \\ D(i\omega) &= \int\frac{dx}{2\pi}\frac{-2\mathrm{Im}D^R(x)}{i\omega-x}, \end{aligned} \tag{24}$$

where the phonon is assumed to be dispersionless for simplicity, which is justified because we are only interested in large phonon momentum. The frequency summation of the intermediate state becomes

$$\begin{aligned} I(\mathbf{q},\mathbf{k},i\Omega) &= \frac{1}{\beta^2}\sum_{i\omega,i\nu} L(\mathbf{q},i\omega)\,L(\mathbf{q}-\mathbf{k},i\omega-i\nu)\,D(i\Omega-i\nu) \\ &= -\frac{1}{\pi^3}\int dxdydz\,\mathrm{Im}L^R(\mathbf{q},x)\,\mathrm{Im}L^R(\mathbf{q}-\mathbf{k},y)\,\mathrm{Im}D^R(z) \\ &\quad\times\frac{1}{\beta^2}\sum_{i\omega,i\nu}\frac{1}{i\omega-x}\frac{1}{i\omega-i\nu-y}\frac{1}{i\Omega-i\nu-z}, \end{aligned} \tag{25}$$

where the last line could be carried out explicitly as follows

$$\frac{1}{\beta^2}\sum_{i\omega,i\nu}\frac{1}{i\omega-x}\frac{1}{i\omega-i\nu-y}\frac{1}{i\Omega-i\nu-z} = \frac{1}{4}\frac{\left(-\coth\frac{x}{2T}+\coth\frac{y}{2T}\right)\left(\coth\frac{x-y}{2T}+\coth\frac{z}{2T}\right)}{i\Omega-x+y-z}. \tag{26}$$

We then perform the analytic continuation of the external frequency $i\Omega\to\Omega+i\delta$, and take the imaginary part of the whole expression. Now the integral contains two delta-functions

$$\begin{aligned} \mathrm{Im}\frac{1}{\Omega-x+y-z+i\delta} &= -\pi\delta(\Omega-x+y-z), \\ \mathrm{Im}D^R(z) &= -\pi\delta(z-\Omega_0)+\pi\delta(z+\Omega_0), \end{aligned} \tag{27}$$

where $\Omega_0$ is the phonon frequency. $\mathrm{Im}I^R(\mathbf{q},\mathbf{k},\Omega)$ could now be written as a one-dimensional integral

$$
\begin{aligned}
\mathrm{Im}I^{R}\left(\mathbf{q},\mathbf{k},\Omega\right) \;=\; & -\frac{1}{\pi}\int dx\,\mathrm{Im}L^{R}\left(\mathbf{q},x\right)\mathrm{Im}L^{R}\left(\mathbf{q}-\mathbf{k},x-\Omega+\Omega_{0}\right)\\
& \times\frac{1}{4}\left(-\coth\frac{x}{2T}+\coth\frac{x-\Omega+\Omega_{0}}{2T}\right)\left(\coth\frac{\Omega-\Omega_{0}}{2T}+\coth\frac{\Omega_{0}}{2T}\right)\\
& -\left\{\Omega_{0}\rightarrow-\Omega_{0}\right\}. \qquad (28)
\end{aligned}
$$

We are interested in the region where $|\Omega-\Omega_0|\ll T$, thus we denote $\delta\Omega=\Omega-\Omega_0$. The frequencies for the two Leggett modes in the integrand are $x$ and $x-\delta\Omega$. Because the Leggett mode has spectral weight only in a small frequency range near $x=0$, we ignore the $\{\Omega_0\rightarrow-\Omega_0\}$ term in the last line. When $\Omega\rightarrow\Omega_0$, $\left|\coth\frac{\Omega-\Omega_0}{2T}\right|\gg\left|\coth\frac{\Omega_0}{2T}\right|$, so we also neglect the $\coth\frac{\Omega_0}{2T}$ term. After these simplifications, we arrive at

$$
\mathrm{Im}I^{R}\left(\mathbf{q},\mathbf{k},\delta\Omega\right) \;=\; \frac{1}{4\pi}\coth\frac{\delta\Omega}{2T}\int dx\,\mathrm{Im}L^{R}\left(\mathbf{q},x\right)\mathrm{Im}L^{R}\left(\mathbf{q}-\mathbf{k},x-\delta\Omega\right)\left(\coth\frac{x}{2T}-\coth\frac{x-\delta\Omega}{2T}\right). \qquad (29)
$$

The above result is to be summed over $\mathbf{q}$ and $\mathbf{k}$, which allows us to make shifts, so that

$$
\begin{aligned}
& \mathrm{Tr}\mathrm{Im}I^{R}\left(\mathbf{q},\mathbf{k},\delta\Omega\right)\\
\rightarrow\; & \frac{1}{4\pi}\coth\frac{\delta\Omega}{2T}\int dx\,\mathrm{Tr}\left[\mathrm{Im}L^{R}\left(\mathbf{q}+\frac{\mathbf{k}}{2},x+\frac{\delta\Omega}{2}\right)\mathrm{Im}L^{R}\left(\mathbf{q}-\frac{\mathbf{k}}{2},x-\frac{\delta\Omega}{2}\right)\right]\left(\coth\frac{x+\frac{\delta\Omega}{2}}{2T}-\coth\frac{x-\frac{\delta\Omega}{2}}{2T}\right)\\
\approx\; & -T^{2}\left(\frac{T}{cN_{0}}\right)^{2}\left(\frac{1}{\Gamma^{(\mathrm{LM})}_{\mathbf{q}+\frac{\mathbf{k}}{2}}}+\frac{1}{\Gamma^{(\mathrm{LM})}_{\mathbf{q}-\frac{\mathbf{k}}{2}}}\right)\frac{1}{\delta\Omega^{2}+\left(\Gamma^{(\mathrm{LM})}_{\mathbf{q}+\frac{\mathbf{k}}{2}}+\Gamma^{(\mathrm{LM})}_{\mathbf{q}-\frac{\mathbf{k}}{2}}\right)^{2}}\\
=\; & -\frac{2T^{4}}{c^{2}N_{0}^{2}}\frac{\tau^{-1}+D\left(q^{2}+k^{2}/4\right)}{\left\{\left[\tau^{-1}+D\left(q^{2}+k^{2}/4\right)\right]^{2}-D^{2}q^{2}k^{2}\cos^{2}\theta\right\}\left\{\delta\Omega^{2}+4\left[\tau^{-1}+D\left(q^{2}+k^{2}/4\right)\right]^{2}\right\}}. \qquad (30)
\end{aligned}
$$

In the derivation we have used $\coth x\approx 1/x$ when $x<1$. Here $\theta$ is the angle between $\mathbf{q}$ and $\mathbf{k}$. The momentum integral then follows

$$
\begin{aligned}
& \frac{1}{V^{2}}\sum_{\mathbf{q},\mathbf{k}}\frac{\tau^{-1}+D\left(q^{2}+k^{2}/4\right)}{\left\{\left[\tau^{-1}+D\left(q^{2}+k^{2}/4\right)\right]^{2}-D^{2}q^{2}k^{2}\cos^{2}\theta\right\}\left\{\delta\Omega^{2}+4\left[\tau^{-1}+D\left(q^{2}+k^{2}/4\right)\right]^{2}\right\}}\\
=\; & 2\pi\int_{0}^{\infty}dx\int_{0}^{\infty}dy\int_{0}^{2\pi}d\theta\frac{\tau^{-1}+D\left(x+y\right)}{\left\{\left[\tau^{-1}+D\left(x+y\right)\right]^{2}-4D^{2}xy\cos^{2}\theta\right\}\left\{\delta\Omega^{2}+4\left[\tau^{-1}+D\left(x+y\right)\right]^{2}\right\}}\\
=\; & 2\pi\int_{0}^{\infty}dx\int_{0}^{2\pi}d\theta\int_{-x}^{+x}dy\frac{\tau^{-1}+\sqrt{2}Dx}{\left\{\left(\tau^{-1}+\sqrt{2}Dx\right)^{2}-2D^{2}\left(x^{2}-y^{2}\right)\cos^{2}\theta\right\}\left\{\delta\Omega^{2}+4\left(\tau^{-1}+\sqrt{2}Dx\right)^{2}\right\}}\\
=\; & \frac{\pi\tau}{D^{2}}\int_{0}^{\infty}dx\int_{0}^{2\pi}d\theta\frac{\arctan\left[\sqrt{\frac{\cos^{2}\theta}{(1+x)^{2}-x^{2}\cos^{2}\theta}}x\right]}{\sqrt{\cos^{2}\theta\left[\left(1+x\right)^{2}-x^{2}\cos^{2}\theta\right]}}\frac{2\left(1+x\right)}{\tau^{2}\delta\Omega^{2}+4\left(1+x\right)^{2}}. \qquad (31)
\end{aligned}
$$

Define a positive weight function

$$
p\left(x\right)=\int_{0}^{2\pi}d\theta\frac{\arctan\left[\sqrt{\frac{\cos^{2}\theta}{(1+x)^{2}-x^{2}\cos^{2}\theta}}x\right]}{\sqrt{\cos^{2}\theta\left[\left(1+x\right)^{2}-x^{2}\cos^{2}\theta\right]}}, \qquad (32)
$$

we have

$$
\mathrm{Im}I^{R}\left(\delta\Omega\right) \;=\; \frac{2\pi}{D^{2}}\frac{T^{4}}{c^{2}N_{0}^{2}}\int_{0}^{\infty}dx\,p\left(x\right)\mathrm{Im}\frac{1}{\delta\Omega+\frac{2i(1+x)}{\tau}}. \qquad (33)
$$

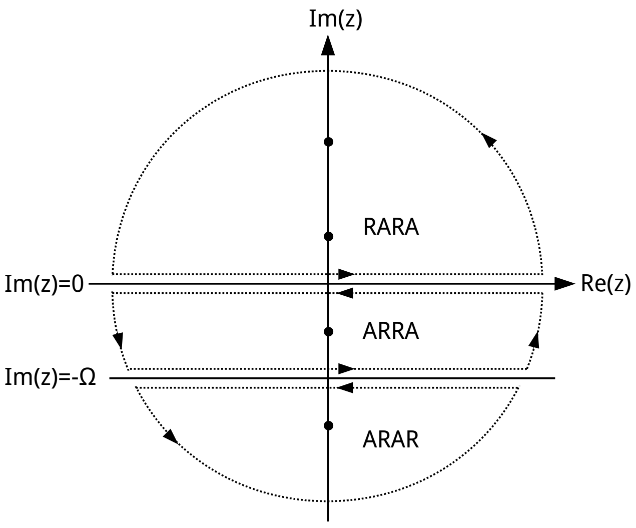


Figure 2: The integration contour. Black dots are the fermionic frequencies, bold black lines are the branch cuts of the integrand ($\Omega$ is a bosonic frequency). R and A denote "retarded" and "advanced" respectively for the four Green's functions in the integrand of equation (37).

Our result is valid for $|\delta\Omega| \ll T$. If we extrapolate the above result to the whole range of $\delta\Omega$, then the Kramers-Kronig relations lead to

$$I^R(\delta\Omega) = \frac{2\pi}{D^2}\frac{T^4}{c^2 N_0^2}\int_0^\infty dx\, p(x)\, \frac{1}{\delta\Omega + \frac{2i(1+x)}{\tau}}. \tag{34}$$

### C. Intermediate state in ordered region $T = 0$

At $T = 0$, the Anderson mode is pushed towards the plasma frequency and is decoupled from the low-energy physics. The only remaining low-lying collective mode is then the Leggett mode, we recall the zero-temperature form of the Leggett mode and the phonon Green's function as follows

$$\begin{aligned} L(\mathbf{q},\omega) &= \frac{4\Delta^2}{N_0}\frac{1}{2\omega_{\mathbf{q}}}\left(\frac{1}{\omega-\omega_{\mathbf{q}}+i\delta} - \frac{1}{\omega+\omega_{\mathbf{q}}-i\delta}\right)\left(\frac{1}{2}-\frac{1}{2}\sigma_x\right), \\ D(\Omega) &= \frac{1}{\Omega-\Omega_0+i\delta} - \frac{1}{\Omega+\Omega_0-i\delta}. \end{aligned} \tag{35}$$

We carry out the frequency integral of the intermediate state by the method of residues

$$\begin{aligned} & \mathrm{Tr} I(\mathbf{q},\mathbf{k},\Omega) \\ &= \int \frac{d\omega}{2\pi i}\frac{d\nu}{2\pi i}\, L(\mathbf{q},\omega)\, L(\mathbf{q}-\mathbf{k},\omega-\nu)\, D(\Omega-\nu) \\ &= \frac{4\Delta^4}{N_0^2}\frac{1}{\omega_{\mathbf{q}}\omega_{\mathbf{q}-\mathbf{k}}}\int \frac{d\omega}{2\pi i}\frac{d\nu}{2\pi i}\left(\frac{1}{\omega-\omega_{\mathbf{q}}+i\delta} - \frac{1}{\omega+\omega_{\mathbf{q}}-i\delta}\right) \\ &\times \left(\frac{1}{\omega-\nu-\omega_{\mathbf{q}-\mathbf{k}}+i\delta} - \frac{1}{\omega-\nu+\omega_{\mathbf{q}-\mathbf{k}}-i\delta}\right)\left(\frac{1}{\Omega-\nu-\Omega_0+i\delta} - \frac{1}{\Omega-\nu+\Omega_0-i\delta}\right) \\ &= \frac{4\Delta^4}{N_0^2}\frac{1}{\omega_{\mathbf{q}}\omega_{\mathbf{q}-\mathbf{k}}}\left[\frac{1}{\Omega-(\Omega_0+\omega_{\mathbf{q}}+\omega_{\mathbf{q}-\mathbf{k}})+i\delta} - \frac{1}{\Omega+(\Omega_0+\omega_{\mathbf{q}}+\omega_{\mathbf{q}-\mathbf{k}})-i\delta}\right]. \end{aligned} \tag{36}$$

### D. Numerical calculation for $B$ in the fluctuation region

With the damping effect, the electron Green's function $G(\mathbf{k}, i\omega \to z)$ has branch-cut on the real-axis $\mathrm{Im}z = 0$. In this case, we do the frequency summation by expanding the contour integral of $z$ around the imaginary axis to infinity, but avoiding the branch-cuts of the integrand as follows (Fig. 2)

$$\begin{aligned}
& \frac{1}{\beta}\sum_{i\omega} G(\mathbf{k}, i\omega)\, G(-\mathbf{k}, -i\omega)\, G(\mathbf{k}+\mathbf{Q}, i\omega + i\Omega)\, G(-\mathbf{k}-\mathbf{Q}, -i\omega - i\Omega) \\
= & \frac{1}{4\pi i}\oint dz \tanh\frac{z}{2T} G(\mathbf{k}, z)\, G(\mathbf{k}, -z)\, G(\mathbf{k}+\mathbf{Q}, z+i\Omega)\, G(\mathbf{k}+\mathbf{Q}, -z-i\Omega) \\
= & \frac{1}{4\pi i}\int dx \tanh\frac{x}{2T} G^R(\mathbf{k}, x)\, G^A(\mathbf{k}, -x)\, G^R(\mathbf{k}+\mathbf{Q}, x+i\Omega)\, G^A(\mathbf{k}+\mathbf{Q}, -x-i\Omega) \\
- & \frac{1}{4\pi i}\int dx \tanh\frac{x}{2T} G^A(\mathbf{k}, x)\, G^R(\mathbf{k}, -x)\, G^R(\mathbf{k}+\mathbf{Q}, x+i\Omega)\, G^A(\mathbf{k}+\mathbf{Q}, -x-i\Omega) \\
+ & \frac{1}{4\pi i}\int dx \tanh\frac{x}{2T} G^A(\mathbf{k}, x-i\Omega)\, G^R(\mathbf{k}, -x+i\Omega)\, G^R(\mathbf{k}+\mathbf{Q}, x)\, G^A(\mathbf{k}+\mathbf{Q}, -x) \\
- & \frac{1}{4\pi i}\int dx \tanh\frac{x}{2T} G^A(\mathbf{k}, x-i\Omega)\, G^R(\mathbf{k}, -x+i\Omega)\, G^A(\mathbf{k}+\mathbf{Q}, x)\, G^R(\mathbf{k}+\mathbf{Q}, -x)\,. \qquad (37)
\end{aligned}$$

In the above equations, $z$ is a complex number and $x$ is a real number. The analytic continuation of the phonon frequency $i\Omega \to \Omega + i\delta$ could then be performed to lead to the following form

$$\begin{aligned}
& B^R(\mathbf{Q}, \Omega) \\
= & \frac{1}{4\pi i}\int \frac{d\mathbf{k}}{(2\pi)^2}\gamma_{\mathbf{k}}\gamma_{\mathbf{k}+\mathbf{Q}}\int dx\ \tanh\frac{x}{2T}\, G^R(\mathbf{k}, x)\, G^A(\mathbf{k}, -x)\, G^R(\mathbf{k}+\mathbf{Q}, x+\Omega)\, G^A(\mathbf{k}+\mathbf{Q}, -x-\Omega) \\
- & \frac{1}{4\pi i}\int \frac{d\mathbf{k}}{(2\pi)^2}\gamma_{\mathbf{k}}\gamma_{\mathbf{k}+\mathbf{Q}}\int dx\ \tanh\frac{x}{2T}\, G^A(\mathbf{k}, x)\, G^R(\mathbf{k}, -x)\, G^R(\mathbf{k}+\mathbf{Q}, x+\Omega)\, G^A(\mathbf{k}+\mathbf{Q}, -x-\Omega) \\
+ & \frac{1}{4\pi i}\int \frac{d\mathbf{k}}{(2\pi)^2}\gamma_{\mathbf{k}}\gamma_{\mathbf{k}+\mathbf{Q}}\int dx\ \tanh\frac{x+\Omega}{2T}\, G^A(\mathbf{k}, x)\, G^R(\mathbf{k}, -x)\, G^R(\mathbf{k}+\mathbf{Q}, x+\Omega)\, G^A(\mathbf{k}+\mathbf{Q}, -x-\Omega) \\
- & \frac{1}{4\pi i}\int \frac{d\mathbf{k}}{(2\pi)^2}\gamma_{\mathbf{k}}\gamma_{\mathbf{k}+\mathbf{Q}}\int dx\ \tanh\frac{x+\Omega}{2T}\, G^A(\mathbf{k}, x)\, G^R(\mathbf{k}, -x)\, G^A(\mathbf{k}+\mathbf{Q}, x+\Omega)\, G^R(\mathbf{k}+\mathbf{Q}, -x-\Omega)\,, \qquad (38)
\end{aligned}$$

where the integral region of $\mathbf{k}$ is restricted to one of the subbands. The final expression is to be calculated numerically. We use the `Cuba library` (`http://www.feynarts.de/cuba/`) to perform the numeric integral. Parameters and results are shown in main text.


[1] Buhmann, J. M., Ossadnik, M., Rice, T. M. & Sigrist, M. Numerical study of charge transport of overdoped $La_{2-x}Sr_xCuO_4$ within semiclassical Boltzmann transport theory. *Phys. Rev. B* **87**, 035129 (2013).

[2] Aslamasov, L. & Larkin, A. The influence of fluctuation pairing of electrons on the conductivity of normal metal. *Physics Letters A* **26**, 238–239 (1968).

[3] Larkin, A. & Varlamov, A. *Theory of Fluctuations in Superconductors* (Oxford Science Publications, 2005).

[4] Leggett, A. J. Number-phase fluctuations in two-band superconductors. *Progress of Theoretical Physics* **36**, 901–930 (1966).

[5] Leggett, A. J. Theory of a superfluid Fermi liquid. II. collective oscillations. *Phys. Rev.* **147**, 119–130 (1966).

[6] Leggett, A. J. Theory of a superfluid Fermi liquid. I. general formalism and static properties. *Phys. Rev.* **140**, A1869–A1888 (1965).
